# Supplementary material for: Nearsightedness of Crystalline Materials and Intergranular Embrittlement
Source: arXiv:2011.08920 source file (2020-11-17)
Supplement: Supplementary file 1 [file SI-arxiv.pdf]

# A Comments on Computational Approach

Central to this investigation is the comparison of Bader atom energies with energies obtained with band methods. While conceptually undemanding, in practice these comparisons introduces sources of computational error. Band determined energies exploit variational methods while Bader atomic energies are calculated via the virial theorem [1, 2, 3]. In the latter case, even small errors in the calculated core electron energies can produce large total energy errors, which may be minimized using all electron methods and large basis sets. In turn, to facilitate comparison of Bader atom and band energies, to the extent possible, the same all electron basis sets and computational framework should be used for both calculations. The Amsterdam Modeling Suite provides the capabilities necessary to address many of these issues.

The suite utilizes the Amsterdam Density Functional (ADF) package [4, 5] to calculate the electronic structure of clusters, and BAND [6, 7, 5] to model extended crystalline systems. Both codes use the same Slater-type-orbital (STO) basis functions, though some of the basis functions available to ADF are not fully supported by BAND, most consequential, the all electron quadruple zeta basis set including four polarization terms (QZ4P).

This became a factor when modeling the $4d$ transition metals where a QZ4P basis set was required to calculate Bader atom energies accurately. Presumably the large basis set was needed due to the greater number of radial nodes and hence more rapidly varying near nucleus charge density. Nonetheless, since BAND calculations could not be converged using the QZ4P basis set a source of computational error was introduced when comparing BAND determined formation energies with Bader atom energies. As a way of estimating the magnitude of this error, ADF was used to calculate single atom and large cluster total energies for all the $4d$ transition metal elements using both the triple zeta including two polarization terms (TZ2P) and QZ4P basis sets. In general, and not surprisingly, the single atom energies were lower for the larger basis set by about 10 eV. For the larger clusters, the total energy per atom was again lower using the QZ4P basis, but this time by about 10.6 eV per atom. Using the difference between the single atom and large cluster total energies as an approximation to the formation energy, the QZ4P basis set yields a more negative formation energy of approximately 0.6 eV per atom.

As a check on the accuracy of Bader atom energies we used the fact that over a Bader atom the integral of $\nabla^2\rho(r)$ should be identically zero [8, 9]. Deviations greater than $10^{-2}$ are deemed marginal and indicative of numerical error. We found that the integrated Laplacian of the charge density over the central Bader atom was sensitive to computational parameters. Best results were achieved with a high density Voronoi integration scheme (accint = 6), "very good" density fitting and an appropriate choice of basis set. Even so, in some circumstances the integral of $\nabla^2\rho(r)$ over the central Bader atom was slightly greater than $10^{-2}$. However, at all times the same value over the central atom and the atoms of its first coordination shell were within acceptable limits. It is for this reason that we monitored the per atom energy of a "central cluster"—the central atom and its nearest neighbor coordination shell–as a function of changing boundary width. All calculations employed the generalized gradient approximation using the Perdew–Burke–Ernzerhof exchange-correlation functional (GGA PBE) [10]. Finally, the BAND calculations used a quadratic tetrahedron method for numerical integration over the Brillouin zone, sampling a minimum of 16 $k$ points in the irreducible wedge.

# B Lattice data

The shell structure for the four lattice types (DC, BCC, HCP, and FCC) discussed in the main text is provided in Tables 1-4 and pictures of representative clusters shown in Figures 1-4.

Table 1: Face-centered cubic (FCC) shell structure. Row 1: Number of the coordination shell. Coordination shell zero is the central atom. Row 2: Number of atoms in coordination shell $n$. Row 3: Total number of atoms in the cluster of $n$ coordination shells. (Hard sphere representations of some of these clusters are provided in the SI.) Row 4: Radius of the cluster, i.e. distance between the central atom and the atoms of the $n^{\text{th}}$ shell in atomic diameters or equivalently nearest neighbor separations.

| **Coordination shell $n$** | **0** | **1** | **2** | **3** | **4** | **5** | **6** | **7** | **8** | **9** | **10** |
|---|---|---|---|---|---|---|---|---|---|---|---|
| Number of $n^{\text{th}}$ neighbors | 1 | 12 | 6 | 24 | 12 | 24 | 8 | 48 | 6 | 48 | 24 |
| Total atoms in cluster | 1 | 13 | 19 | 43 | 55 | 79 | 87 | 135 | 141 | 189 | 213 |
| Cluster radius | 0 | 1 | $\sqrt{2}$ | $\sqrt{3}$ | 2 | $\sqrt{5}$ | $\sqrt{6}$ | $\sqrt{7}$ | $2\sqrt{2}$ | 3 | $\sqrt{10}$ |

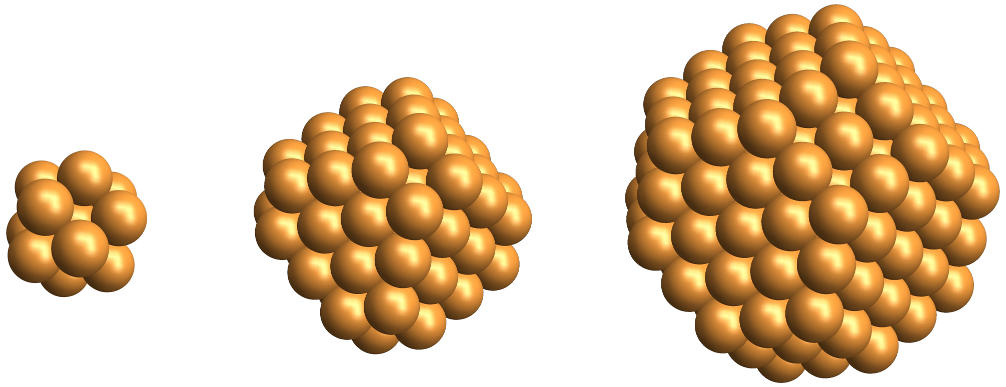

Figure 1: The FCC central 13-atom cluster (left), critical cluster consisting of 5 coordination shells (middle), and the largest cluster consisting of 10 coordination shells (right).

Table 2: Body-centered cubic (BCC) shell structure. Table layout is identical to that of Table 1.

| **Coordination shell $n$** | **0** | **1** | **2** | **3** | **4** | **5** | **6** | **7** | **8** | **9** | **10** |
|---|---|---|---|---|---|---|---|---|---|---|---|
| Number of $n^{\text{th}}$ neighbors | 1 | 8 | 6 | 12 | 24 | 8 | 6 | 24 | 24 | 24 | 8 |
| Total atoms in cluster | 1 | 9 | 15 | 27 | 51 | 59 | 65 | 89 | 113 | 137 | 145 |
| Cluster radius | 0 | 1 | $2\sqrt{\frac{1}{3}}$ | $2\sqrt{\frac{2}{3}}$ | $\sqrt{\frac{11}{3}}$ | 2 | $4\sqrt{\frac{1}{3}}$ | $\sqrt{\frac{19}{3}}$ | $2\sqrt{\frac{5}{3}}$ | $2\sqrt{2}$ | 3 |

Table 3: Hexagonal close-packed (HCP) shell structure. Table layout is identical to that of Table 1.

| **Coordination shell $n$** | **0** | **1** | **2** | **3** | **4** | **5** | **6** | **7** | **8** | **9** | **10** | **11** |
|---|---|---|---|---|---|---|---|---|---|---|---|---|
| Number of $n^{\text{th}}$ neighbors | 1 | 12 | 6 | 2 | 18 | 12 | 6 | 12 | 12 | 6 | 3 | 12 |
| Total atoms in cluster | 1 | 13 | 19 | 21 | 39 | 51 | 57 | 69 | 81 | 87 | 90 | 102 |
| Cluster radius | 0 | 1 | $\sqrt{2}$ | $2\sqrt{\frac{2}{3}}$ | $\sqrt{3}$ | $\sqrt{\frac{11}{3}}$ | 2 | $\sqrt{5}$ | $\sqrt{\frac{17}{3}}$ | $\sqrt{6}$ | $\sqrt{\frac{19}{3}}$ | $2\sqrt{\frac{5}{3}}$ |

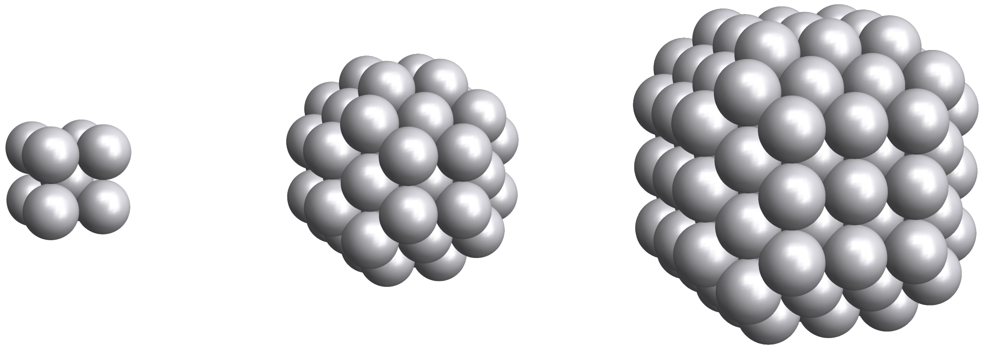

Figure 2: The BCC central 9-atom cluster (left), critical cluster consisting of 5 coordination shells (middle), and the largest cluster consisting of 10 coordination shells (right).

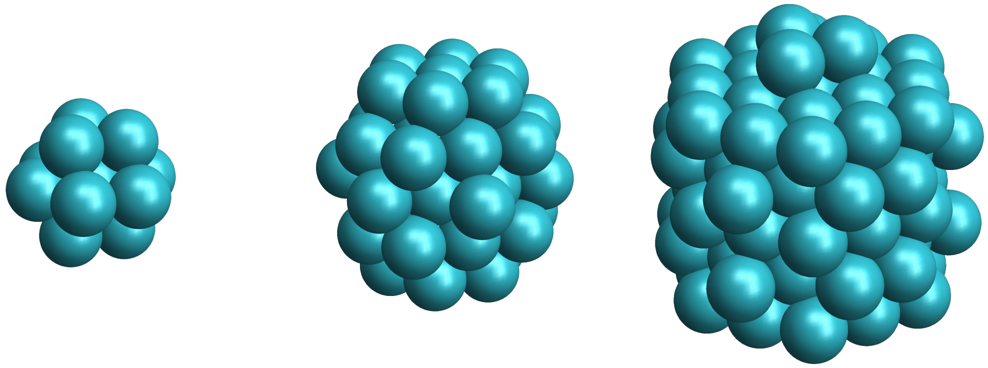

Figure 3: The HCP central 13-atom cluster (left), critical cluster consisting of 5 coordination shells (middle), and the largest cluster consisting of 11 coordination shells (right).

Table 4: Diamond cubic (DC) shell structure. Table layout is identical to that of Table 1.

| **Coordination shell $n$** | **0** | **1** | **2** | **3** | **4** | **5** | **6** | **7** | **8** | **9** | **10** | **11** |
|---|---|---|---|---|---|---|---|---|---|---|---|---|
| Number of $n^{\text{th}}$ neighbors | 0 | 4 | 12 | 12 | 6 | 12 | 24 | 16 | 12 | 24 | 12 | 8 |
| Total atoms in cluster | 1 | 5 | 17 | 29 | 35 | 47 | 71 | 87 | 99 | 123 | 135 | 143 |
| Cluster radius | 0 | 1 | $2\sqrt{\frac{2}{3}}$ | $\sqrt{\frac{11}{3}}$ | $4\sqrt{\frac{1}{3}}$ | $\sqrt{\frac{19}{3}}$ | $2\sqrt{2}$ | 3 | $4\sqrt{\frac{2}{3}}$ | $\sqrt{\frac{35}{3}}$ | $\sqrt{\frac{43}{3}}$ | 4 |

## C Element data

Data from which the graphs shown in the main text were constructed are provided in Tables 5-8.

Table 5: Perturbation energies $\Delta E$ of the (single) DC cluster investigated, reported in eV.

| **Element** | **Diameter (Å)** | $E_f$ | $E_0$ | $\Delta E_1$ | $\Delta E_2$ | $\Delta E_3$ | $\Delta E_4$ | $\Delta E_5$ | $\Delta E_6$ | $\Delta E_7$ | $\Delta E_8$ | $\Delta E_9$ | $\Delta E_{11}$ |
|---|---|---|---|---|---|---|---|---|---|---|---|---|---|
| Si | 2.352 | -5.42 | -7865.72 | -3.05 | -9.01 | -5.66 | -5.55 | -6.09 | -6.71 | -6.67 | -6.12 | -5.91 | -5.79 |

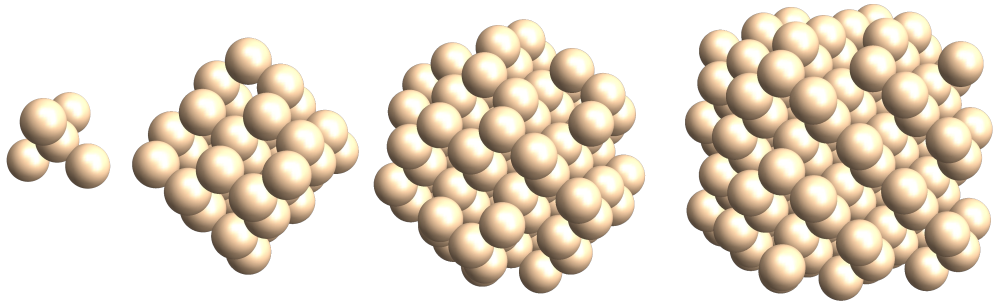

Figure 4: (from the left) The DC central 5-atom cluster, the 4-coordination cluster closing the central atom, the 7-coordination cluster closing the central cluster, and the largest cluster consisting of 11 coordination shells.

Table 6: Perturbation energies $\Delta E$ of FCC clusters, reported in eV.

| **Element** | **Diameter (Å)** | $E_f$ | $E_0$ | $\Delta E_1$ | $\Delta E_2$ | $\Delta E_3$ | $\Delta E_4$ | $\Delta E_5$ | $\Delta E_6$ | $\Delta E_7$ | $\Delta E_9$ |
|---|---|---|---|---|---|---|---|---|---|---|---|
| Al | 2.864 | -3.78 | -6587.00 | -8.80 | -5.86 | -7.20 | - | -4.65 | - | -3.48 | -4.08 |
| Cu | 2.553 | -3.54 | -44611.75 | -3.64 | -5.66 | -3.83 | - | -4.37 | - | -3.56 | -3.56 |
| Rh | 2.758 | -6.78 | -127504.31 | -3.05 | -4.00 | -5.87 | - | -6.32 | - | -7.08 | - |
| Pd | 2.751 | -3.99 | -134362.32 | -1.52 | -2.22 | -4.07 | - | -4.71 | - | -4.88 | - |
| Ag | 2.885 | -3.71 | -141429.58 | -1.38 | -2.13 | -3.83 | - | -3.90 | - | -4.01 | - |

Table 7: Perturbation energies $\Delta E$ of BCC clusters, reported in eV.

| **Element** | **Diameter (Å)** | $E_f$ | $E_0$ | $\Delta E_1$ | $\Delta E_2$ | $\Delta E_3$ | $\Delta E_4$ | $\Delta E_5$ | $\Delta E_6$ | $\Delta E_7$ | $\Delta E_8$ | $\Delta E_{10}$ |
|---|---|---|---|---|---|---|---|---|---|---|---|---|
| V | 2.624 | -8.36 | -25665.42 | -3.45 | -4.35 | -7.60 | -8.99 | -8.74 | -8.82 | -9.33 | -9.04 | -8.95 |
| Nb | 2.857 | -10.22 | -102139.80 | -2.77 | -4.06 | -8.71 | -9.39 | -10.93 | -11.02 | -11.00 | -11.06 | - |
| Mo | 2.725 | -10.29 | -108177.90 | -1.57 | -9.08 | -8.29 | -8.82 | -10.16 | -10.15 | -11.51 | -11.06 | - |

Table 8: Perturbation energies $\Delta E$ of HCP clusters, reported in eV.

| **Element** | **Diameter (Å)** | $E_f$ | $E_0$ | $\Delta E_1$ | $\Delta E_2$ | $\Delta E_3$ | $\Delta E_4$ | $\Delta E_5$ | $\Delta E_6$ | $\Delta E_7$ | $\Delta E_9$ | $\Delta E_{11}$ |
|---|---|---|---|---|---|---|---|---|---|---|---|---|
| Tc | 2.735 | -11.52 | -114414.78 | -3.95 | -4.87 | - | -9.30 | -10.70 | - | -11.85 | -12.06 | -12.52 |
| Ru | 2.706 | -9.79 | -120855.98 | -4.66 | -5.07 | - | -8.67 | -9.78 | - | -10.84 | -11.10 | -11.37 |

# D Cu-Bi grain boundary data

Grain boundaries are 2-dimensional defects that are present in real materials. They form the interface that separates the orientation in which atoms are stacked; and alter the microstructure, thus affecting performance. The data represented in graphical form in main text is provided in Table 9 and pictures of important clusters in Figure 5/

Table 9: Perturbation energies $\boldsymbol{\Delta E}$ to the 14 atom first coordination shell surrounding the copper or bismuth atom at the center in the $\Sigma 5$ grain boundary clusters Row 1: Number of atoms in the cluster. Row 2: Cluster radii in units of Å. Row 3: per atom energies of central cluster with Bi at center in eV – relative to isolated central cluster. Row 4: per atom energies of central cluster with Cu at center in eV – relative to isolated central cluster.

| **Number of atoms in cluster** | **Cluster radii (Å)** | **$\Delta E$ with Bi (eV/atom)** | **$\Delta E$ with Cu (eV/atom)** |
|---|---|---|---|
| 15 | 2.906 | 0.00 | 0.00 |
| 23 | 4.280 | -2.89 | 0.14 |
| 31 | 4.638 | -5.12 | -0.39 |
| 39 | 4.683 | -6.55 | -0.55 |
| 47 | 4.812 | -7.61 | -0.54 |
| 55 | 5.444 | -8.66 | -0.54 |
| 63 | 5.725 | -9.16 | -0.40 |
| 71 | 5.764 | -9.32 | -0.10 |
| 77 | 5.893 | -9.22 | 0.28 |
| 83 | 6.528 | -9.39 | 0.38 |
| 93 | 6.817 | -9.70 | 0.41 |
| 97 | 6.873 | -9.67 | 0.44 |

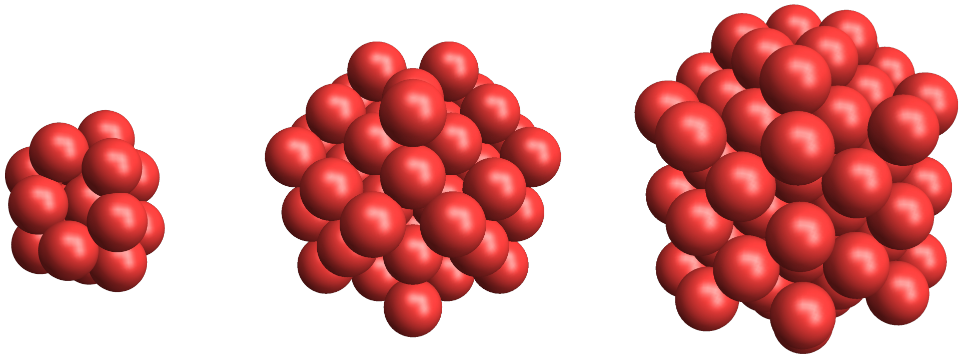

Figure 5: The grain boundary central 15-atom cluster (left), critical cluster consisting of 63 atoms (middle), and the largest cluster consisting of 97 atoms (right).

# References


[1] J. C. Slater. The Virial and Molecular Structure. *The Journal of Chemical Physics*, 1(10):687–691, 1933.

[2] Klaus Ruedenberg and Michael W. Schmidt. Physical Understanding through Variational Reasoning: Electron Sharing and Covalent Bonding. *The Journal of Physical Chemistry A*, 113(10):1954–1968, 2009.

[3] Juan I. Rodríguez, Paul W. Ayers, Andreas W. Götz, and F. L. Castillo-Alvarado. Virial theorem in the kohn–sham density-functional theory formalism: Accurate calculation of the atomic quantum theory of atoms in molecules energies. *The Journal of Chemical Physics*, 131(2):021101, 2009.

[4] G te Velde, F M Bickelhaupt, E J Baerends, C Fonseca Guerra, S J A van Gisbergen, J G Snijders, and T Ziegler. Chemistry with ADF. *Journal of Computational Chemistry*, 22(9):931–967, 2001.

[5] E J Baerends, T Ziegler, A J Atkins, J Autschbach, D Bashford, A Bérces, F M Bickelhaupt, C Bo, P M Boerrigter, L Cavallo, D P Chong, D V Chulhai, L Deng, R M Dickson, J M Dieterich, D E Ellis, M van Faassen, L Fan, T H Fischer, C Fonseca Guerra, M Franchini, A Ghysels, A Giammona, S J A van Gisbergen, A W Götz, J A Groeneveld, O V Gritsenko, M Grüning, S Gusarov, F E Harris, P van den Hoek, C R Jacob, H Jacobsen, L Jensen, J W Kaminski, G van Kessel, F Kootstra, A Kovalenko, M V Krykunov, E van Lenthe, D A McCormack, A Michalak, M Mitoraj, S M Morton, J Neugebauer, V P Nicu, L Noodleman, V P Osinga, S Patchkovskii, M Pavanello, C A Peeples, P H T Philipsen, D Post, C C Pye, W Ravenek, J I Rodríguez, P Ros, R Rüger, P R T Schipper, H van Schoot, G Schreckenbach, J S Seldenthuis, M Seth, J G Snijders, M Solà, M Swart, D Swerhone, G te Velde, P Vernooijs, L Versluis, L Visscher, O Visser, F Wang, T A Wesolowski, E M van Wezenbeek, G Wiesenekker, S K Wolff, T K Woo, and A L Yakovlev. *ADF2016, SCM, Theoretical Chemistry, Vrije Universiteit, Amsterdam, The Netherlands.* 2016.

[6] G. te Velde and E.J. Baerends. Precise density-functional method for periodic structures. *Physical Review B*, 44:7888, 1991.

[7] G. Wiesenekker and E.J. Baerends. Quadratic integration over the three-dimensional brillouin zone. *Journal of Physics: Condensed Matter*, 3:6721, 1991.

[8] R. F. W. Bader. *Atoms in Molecules: A Quantum Theory.* Clarendon Press: Oxford, UK, 1990.

[9] C. F. Matta and R. J. Boyd, editors. *The Quantum Theory of Atoms in Molecules: From Solid State to DNA and Drug Design.* Wiley-VCH Verlag GmbH & Co. KGaA: Weinheim, 2007.

[10] John P. Perdew, Kieron Burke, and Matthias Ernzerhof. Generalized gradient approximation made simple. *Phys. Rev. Lett.*, 77:3865–3868, Oct 1996.
